# Supplementary material for: On the accuracy of self-normalized log-linear models
Source: arXiv:1506.04147 source file (2015-06-18)
Supplement: Supplementary file 1 [file supplement.tex]

17 gid=649427843
18 uid=1805499484
20 ctime=1433349572
20 atime=1434130806
23 SCHILY.dev=16777220
23 SCHILY.ino=54621280
18 SCHILY.nlink=1
